# Supplementary material for: Tuneable entangled photon pair generation in a liquid crystal
Source: arXiv:2401.07362 source file (2024-06-02)
Supplement: Supplementary file 1 [file methods+supp.pdf]

## METHODS AND SUPPLEMENTARY

### MATERIAL AND SAMPLE PREPARATION

The material employed in this study is FNLC-1751 supplied by Merck Electronics KGaA. FNLC-1751 shows a stable ferroelectric nematic phase at room temperature, with the phase sequence Iso –  $87^{\circ}\text{C}$  N –  $57^{\circ}\text{C}$  - M2 -  $45^{\circ}\text{C}$  – NF on cooling, where N refers to the non-polar nematic phase, M2 to the so-described splay modulated antiferroelectric nematic phase [1–3] and NF to the ferroelectric nematic phase.

The material was confined in glass LC cells, which were filled by capillary forces at  $100^{\circ}\text{C}$  in the isotropic phase. Two kinds of cells were employed, commercially available ones and homemade. In the latter case soda lime glass square  $2\text{ cm} \times 2\text{ cm}$  plates coated with transparent ITO conductive layer were assembled with plastic beads (EPOSTAR) spacers in order to achieve a variety of cells with different thicknesses ranging from  $5\text{--}8\text{ }\mu\text{m}$ . In the bottom glass  $500\text{ }\mu\text{m}$  slit was etched in the ITO coating in order to apply in-plane fields. Additionally, both plates were treated with a 30% solution of polyimide SUNEVER 5291 (Nissan) film and subsequently rubbed in order to achieve orientational in-plane anchoring (planar alignment) of the liquid crystal. Combinations of different relative rubbing directions of the top and bottom glass plates ( $0^{\circ}$ ,  $90^{\circ}$  or  $180^{\circ}$ ) result in different twist structures of the liquid crystal sample in the ferroelectric nematic phase [4–6]. In the three cases rubbing in the electrode gap glass was performed along the gap. Two different commercially available cells were also employed. For experiments on uniform structures,  $5\text{ }\mu\text{m}$  EHC D-type cells with parallel rubbed surfaces (aligning agent polyimide LX-1400 from Hitachi-Kasei) were used. In-plane switching (IPS) LC cells purchased from Instec were employed for switching experiments on  $180^{\circ}$ -twisted structures. Cells have in one of the substrates interdigitated electrodes with alternating polarity and an electrode width and gap between them of  $15\text{ }\mu\text{m}$ . Cell thickness was  $9\text{ }\mu\text{m}$ . Surfaces have antiparallel rubbing along the electrodes (aligning agent KPI300B).

After filling, the sample was brought to room temperature by controllably decreasing the temperature at a rate of  $0.5^{\circ}\text{C}/\text{min}$ . In the case of initially large domains breaking down into smaller ones after the application of large voltages, initial configuration was restored by reheating the samples and subsequent controlled cooling back to room temperature.

### ELECTRIC FIELD SWITCHING AND POLARIZATION MICROSCOPY

To measure the structure of the samples and the structural changes upon applying electric field samples were analyzed in terms of polarization microscopy. The samples were analyzed with an optical microscope (Nikon Ti2) used in transmission regime with white LED as a source and a set of crossed polarizers on both sides of the sample. A color camera (IDS) with  $2456 \times 2054$  pixels and pixel size of  $3.45\text{ }\mu\text{m}$  was used to acquire the images. For applying the electric field a functional generator was used. Typical voltages that were applied were in the range of  $0.5\text{--}2\text{ V}$ . Both square and ramp voltage as a function of time was tested on the samples.

## SECOND HARMONIC GENERATION

For measuring Second-Harmonic Generation (SHG) the samples were pumped with an optical-parametric oscillator (OPO) tunable laser (OPOTEK Opolette 355) at 850 nm. The laser with 5 ns pulses and 20 Hz repetition rate. The energy of the pulses was typically in the range between 50–100  $\mu$ J. A long-pass filter with the edge at 800 nm was used to filter out any SHG signal generated in the OPO. Pump beam was focused on the sample through a 50/50 beamsplitter and 10x, 0.3 NA objective (Nikon), which was also used to gather the reflected light consisting of both reflected laser light and generated SHG. A shortpass filter at 550 nm was used to reject the reflected laser light. The collected light was analyzed by an imaging spectrometer (Andor Shamrock SR-500i) with a 15  $\mu$ m wide slit, a grating with 300 lines per mm and a CCD detector with a resolution of 1600 pixels. Typical exposure times were 0.5–2 s.

## DETERMINING $\chi^{(2)}$

Determining the shape of the  $\chi^{(2)}$  tensor was based upon the measurement of SHG at different combinations of polarizer and analyzer relative orientations. Linearly polarized femtosecond pump laser (Menlo Systems CFiber A 780, 785 nm, 100 fs, 100 MHz, 30 mW pump power at the sample) was sent through a half-waveplate serving as a rotating polarizer. The waveplate was continuously rotated from 0 to  $\pi/2$  at three different positions of the analyzer, namely 0,  $\pi/2$  and  $\pi/4$  (horizontal, vertical and diagonal polarization respectively), relatively to the 0 of the rotating waveplate, corresponding to the orientation of the molecules long axis. Based on the intrinsic simetry and reshaping  $\chi^{(2)}$  into the effective tensor  $d$ , the relation between the pump and SHG electric field becomes

$$\begin{pmatrix} E_{\parallel} \\ E_o \\ E_e \end{pmatrix}_{SHG} = \begin{pmatrix} d_{11} & d_{12} & d_{13} & d_{14} & d_{15} & d_{16} \\ d_{21} & d_{22} & d_{23} & d_{24} & d_{25} & d_{26} \\ d_{31} & d_{32} & d_{33} & d_{34} & d_{35} & d_{36} \end{pmatrix} \begin{pmatrix} E_{\parallel}^2 \\ E_o^2 \\ E_e^2 \\ 2E_oE_e \\ 2E_{\parallel}E_e \\ 2E_{\parallel}E_o \end{pmatrix}_{PUMP}$$

where indices  $\parallel$ ,  $e$  and  $o$  denote directions along the sample, along the molecules extraordinary and along ordinary axis, respectively. Transverse electric field propagating in  $\parallel$  direction can be written as

$$E = E_0 \begin{pmatrix} \cos\theta \\ \sin\theta \end{pmatrix},$$

where  $\theta$  denotes the polarization angle of the pump with respect to the molecules orientation. The SHG intensity for the selected three analyzer orientations can be written as

$$\begin{aligned}\frac{I_H^{SHG}}{I_0^2} &= [d_{33}\cos^2\theta + d_{32}\sin^2\theta + 2d_{34}\cos\theta\sin\theta]^2 \\ \frac{I_V^{SHG}}{I_0^2} &= [d_{23}\cos^2\theta + d_{22}\sin^2\theta + 2d_{24}\cos\theta\sin\theta]^2 \\ \frac{I_D^{SHG}}{I_0^2} &= \frac{1}{2} [(d_{33} + d_{23})\cos^2\theta + (d_{32} + d_{22})\sin^2\theta + 2(d_{34} + d_{24})\cos\theta\sin\theta]^2.\end{aligned}$$

These equations were fitted to the results. In first and second equation a set of three components appear independently so their relative intensities can be compared, while in the third equation both two sets are present so the relative intensities of the two sets can be compared. At the end, we obtain the values of the components normalized to the strongest component  $d_{33}$ . The actual equations used for fitting were additionally modified due to the sample birefringence. This correction was performed by multiplying both the  $E$  field vector of the pump and of SHG with a corresponding Jones matrix.

## REFRACTIVE INDEX MEASUREMENT

To measure the extraordinary and ordinary components of the refractive index as well as their dispersion the material was dropcasted on the imaging slide of an Abbe refractometer. No aligning layer was used to orient the sample. The sample was left to stabilize on the refractometer for one day before proceeding with the measurements. A set of narrow bandpass filters with 10 nm bandwidth were used to measure the refractive index values at different wavelengths. The ordinary value of the refractive index was estimated from the lower index boundary line while the extraordinary value is estimated for the orthogonal incoming light polarization from the higher index boundary gradient. Birefringence was additionally and independently measured via the wedge cell method at different wavelengths and is consistent with the birefringence calculated from the values for ordinary and extraordinary refractive index obtained with the Abbe refractometer. To determine also the values outside of the visible wavelength range, namely in the infrared region, a two-term form of Cauchy model was fitted to the data. The fit results in the following values for the Cauchy parameters:  $A = 1.663$ ,  $B = 10256$  for extraordinary refractive index and  $A = 1.474$ ,  $B = 874$  for ordinary refractive index.

## SPDC IN LIQUID CRYSTALS - THEORETICAL MODEL

Here the theoretical derivation of the polarization state of SPDC photons generated from a twisted liquid crystal cell is presented. This can be used to calculate the polarization state (a.k.a the coefficients of the polarization state wavefunction) for a given sample configuration, namely different twist angles and cell thicknesses as well as for different pump polarization with respect to the molecular axis at the beginning of the sample. Other parameters (components of anisotropy tensor, birefringence and the values of refractive index, wavelengths etc.) are fixed so far based on the properties of the current samples used in experiments, but could in principle also be tuned to produce the desired state.

The derivation starts by writing down the dipole interaction between light and matter from which

the interaction part of the Hamiltonian will follow. Within dipole approximation, interaction can be written as

$$H = -\vec{d} \cdot \vec{E}, \quad (1)$$

where  $\vec{E}$  is the electric field and  $\vec{d}$  is the dipole moment that, for continuous mater, can be written in terms of polarization as

$$\vec{d} = \int d^3\vec{r} \vec{P}. \quad (2)$$

Polarization of the medium consists of linear and nonlinear terms and can be written (up to the second term) as

$$\vec{P} = \epsilon_0 \chi^{(1)} \vec{E} + \epsilon_0 \chi^{(2)} \vec{E} \vec{E}. \quad (3)$$

Therefore the energy can be written as

$$H = H_{NL} = -\epsilon_0 \int d^3\vec{r} \chi^{(2)} \vec{E} \vec{E} \vec{E}, \quad (4)$$

where only the nonlinear term is studied, as it will be the interaction part of the hamiltonian describing SPDC. The next step is to introduce quantum description of the quantities (operators) meaning that the energy  $H$  will be replaced with a Hamiltonian  $\hat{H}$ . In order to do so, electric fields need to be replaced with their corresponding operators. Quantization of EM field leads to the following operator of the electric field

$$\hat{E} = \sum_{\mu} \int_{V_q} V_q^{1/2} d^3\vec{k} \left( \frac{\hbar\omega}{2\epsilon_0} \right)^{1/2} \left[ i \hat{a}_{\vec{k},\mu} \vec{e}_{\vec{k},\mu} e^{i(\vec{k}\vec{r}-\omega t)} + \text{h.c.} \right], \quad (5)$$

where the field is written as the Fourier transform in the basis of plane waves. The integral and the sum go over all possible modes (i.e. all wavectors  $\vec{k}$  and polarizations states  $\mu$ , respectively) and  $V_q$  is the quantization volume (space where all  $\vec{k}$  modes exist),  $\vec{e}$  is the unit vector defining the direction (polarization), and  $\hat{a}$  (and its hermitian conjugated counterpart  $\hat{a}^\dagger$ ) is the annihilation (creation) operator that annihilates (creates) a photon in a given state:

$$\hat{a}_{\vec{k},\mu} |n_{\vec{k},\mu}\rangle = \sqrt{n} | (n-1)_{\vec{k},\mu} \rangle, \quad (6)$$

$$\hat{a}_{\vec{k},\mu}^\dagger |n_{\vec{k},\mu}\rangle = \sqrt{n+1} | (n+1)_{\vec{k},\mu} \rangle, \quad (7)$$

where  $n$  denotes the number of photons in a given state. The calculations are performed in the so-called collinear regime, where all three photons propagate in the same direction. For that reason, alongside the phase matching condition (momentum conservation), the Fourier integral in  $k$  space, which brings the angular dependence, can be left out and only the term with  $\omega$  remains out of the plane waves (i.e. the absolute value of  $k$  vector) giving us the spectral dependence.

Since SPDC is an extremely weak process, the pump beam is negligibly affected by the interaction. Therefore the electric field of the pump  $\vec{E}_p$  can be treated classically and will be written as

$$\vec{E}_p = A(x, y) \vec{e}_p e^{-i\omega_p t}, \quad (8)$$

where the assumption that the pump beam amplitude is constant along the propagation ( $z$ ) is made, which is reasonable in the case of thin samples. This leads to the following version of the hamiltonian, where  $p$ ,  $s$  and  $i$  denote pump, signal and idler, respectively

$$\hat{H} = -\epsilon_0 \int d^3\vec{r} \chi^{(2)} \hat{E}_s \hat{E}_i \vec{E}_p. \quad (9)$$

Based on equations (5) and (8) this can be written as

$$\hat{H} = K(x, y, \omega) \sum_{\mu, \mu'} \int dz \chi^{(2)} \vec{e}_s^* \vec{e}_i^* \vec{e}_p \hat{a}_s^\dagger \hat{a}_i^\dagger. \quad (10)$$

This expression needs some additional explanation. Since the interest is the polarization state, all non-polarization dependence can be written in terms of a constant  $K$  which will be the same for all polarization components in the wavefunction and will only define the absolute intensity (i.e. generation efficiency). So only the term of the hamiltonian responsible for generating different polarization states is left in the expression. Moreover, only the hermite conjugate part of expression (5) is taken into account as the other part will not contribute to the creation of photon pairs. Additionally, the relevant part of integration is along  $z$  (which is defined as the coordinate in the direction of propagation, i.e. normal to the sample). Due to birefringence and molecular twist both  $\chi^{(2)}$  and the polarizations of the photons are changing along  $z$  while assumption that they are constant in the lateral directions ( $x$  and  $y$ ) is made. Lastly,  $\hat{a}_s^\dagger$  and  $\hat{a}_i^\dagger$  denote the creation operators of signal and idler photon in a given polarization state ( $\mu, \mu'$ ).

The wavefunction is written in terms of time evolution following Schrödinger equation.

$$i\hbar \frac{d}{dt} |\Psi\rangle = \hat{H} |\Psi\rangle, \quad (11)$$

The time evolution of the state can be written as

$$|\Psi\rangle = e^{\frac{1}{i\hbar} \int \hat{H} dt} |\Psi\rangle_0. \quad (12)$$

Since SPDC interaction is weak the exponential term can be written in terms of Taylor expansion up to the first two terms

$$|\Psi\rangle \approx |vac\rangle + \frac{t}{i\hbar} \hat{H} |vac\rangle, \quad (13)$$

where the vacuum state ( $|vac\rangle$ ) is defined as the initial state without any SPDC photons and it is assumed that  $\hat{H}$  is time-independent. Following from equation (10), the wavefunction can be written by applying the creation operators (in H, V basis) as

$$|\Psi\rangle = c_1\sqrt{2}|HH\rangle + c_2|HV\rangle + c_3\sqrt{2}|VV\rangle. \quad (14)$$

The  $|vac\rangle$  state is neglected as it is irrelevant. Since the two photons are indistinguishable,  $|HV\rangle$  and  $|VH\rangle$  are not considered as separate states. The  $\sqrt{2}$  in the first and third term comes from applying the creation operator on the same state twice (see eq. 7). The coefficients  $c_1, c_2, c_3$  are defined from the integral of the convolution of  $\chi^{(2)}$  tensor with the polarization basis vectors of pump, signal and idler photons:

$$\int dz \chi^{(2)} \vec{e}_s^* \vec{e}_i^* \vec{e}_p. \quad (15)$$

This expression will be evaluated later in the derivation and in the last step the terms with the same basis vectors will be grouped to yield the corresponding coefficients  $c_1, c_2, c_3$ .

So the main thing that needs to be evaluated is the convolution. Instead of  $\chi^{(2)}$  tensor, the standard notation of Kleinman  $d$  tensor is introduced, thus the convolution is written as

$$\chi^{(2)} \vec{e}_s^* \vec{e}_i^* \vec{e}_p = e_s^{o*} e_i^{o*} (d_{22} e_p^o + d_{32} e_p^e) + e_s^{e*} e_i^{e*} (d_{23} e_p^o + d_{33} e_p^e) + (e_s^{e*} e_i^{o*} + e_s^{o*} e_i^{e*}) (d_{24} e_p^o + d_{34} e_p^e), \quad (16)$$

where the polarization basis vectors and the tensor components are functions of  $z$  and the convolution is defined in the local coordinate system of the molecules where  $e$  denotes extraordinary (index 3 of  $d$  tensor) and  $o$  ordinary axis (index 2 of  $d$  tensor). Other terms would couple basis vectors in  $z$  direction which are non-existing in this case due to having transverse waves. Description with two coordinate systems will be swapping throughout the derivation. First is the global coordinate system in which the polarization of the pump and the end polarization of photon pairs (the polarization when exiting the medium) will be written. In this system,  $H$  direction will be defined along  $x$  coordinate and  $V$  along  $y$  coordinate, while  $z$  will be the direction of propagation. The second is the local coordinate system which is defined by the orientation of the molecules, namely so that  $x$  is along the extraordinary axis of the molecules (denoted as  $e$ ) and  $y$  along the ordinary axis ( $o$ ), while  $z$  coordinate denotes the same direction in both systems. The local coordinate system will be changing across the sample, following the twist of the molecules. The purpose of two coordinate systems is that the generated state of photon pairs needs to be written in global coordinate system, while the convolution of the  $\chi^{(2)}$  tensor with the polarization unit vectors has to be performed in the local coordinate system of the molecules as in equation (16).

The polarization of the pump as well as of the generated pairs is changing along the sample due to birefringence and twist. This transformation will be different for each source of pairs (i.e. for every position  $z$  where the photons are generated). In order to calculate the state, all of them need to be taken into account. For this reason, the sample can be represented as a series of infinitely thin slices and the state generated in each of them is calculated, followed by the summation from all of the slices (i.e. interference). This is exactly what the integral of convolution (eq. 15) represents, but to evaluate it, first, the polarization transformation along the sample for pump, signal and idler has to be calculated.

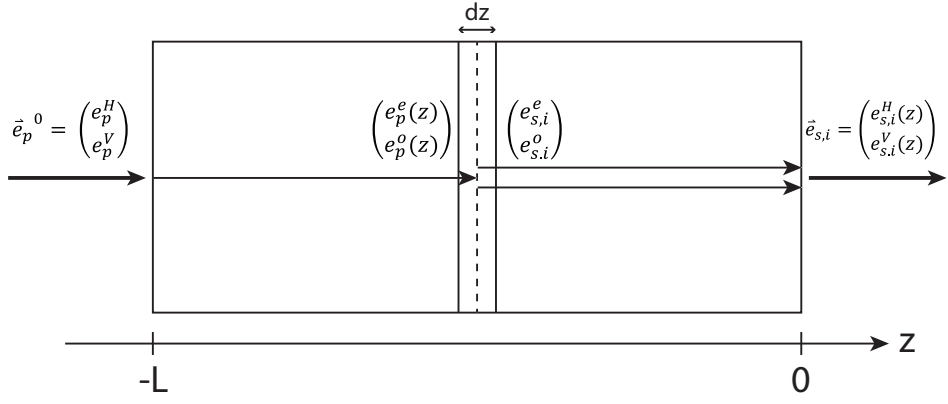

**Figure 1:** Propagation within the sample.

The idea of the calculation is illustrated in figure 1. The state generated by every slice  $dz$  along the sample has to be calculated. First, the pump has to be propagated from  $-L$  to  $z$  and its polarization transformation has to be calculated, and then the generated signal and idler photons have to be propagated from  $z$  to  $0$  and their polarization transformation needs to be calculated. Lastly, the integration for all the slices is performed (i.e. account for the net contribution of the entire sample).

The first step, therefore, is to calculate the propagation of the pump. Initial pump polarization is represented as a Jones vector (fig. 1) in  $H, V$  basis. The angle  $\varphi_0$  is defined as the angle between both coordinates systems at the beginning of the sample, i.e. the angle between the global coordinate  $H$  direction and extraordinary molecule axis  $e$  at the beginning of the sample. In order to write the pump polarization in local coordinate system, the first step is, therefore, to rotate it by this angle:

$$\vec{e}_p^{in} = R(\varphi_0) \vec{e}_p^0, \quad (17)$$

where  $R$  is the standard rotation matrix. In order to propagate the polarization along the sample, the right Jones matrix has to be applied. Jones matrix for a twisted nematic liquid crystal is known [7–9] and can be written as

$$M_{TLC} = e^{i\phi} R(-\varphi) M(\varphi, \beta) \quad M(\varphi, \beta) = \begin{pmatrix} \cos X + i\frac{\beta}{X} \sin X & \frac{\varphi}{X} \sin X \\ -\frac{\varphi}{X} \sin X & \cos X - i\frac{\beta}{X} \sin X \end{pmatrix} \quad (18)$$

The parameters used are  $\phi = \tilde{k}l$ , where  $\tilde{k} = \frac{1}{2}(k^e + k^o)$  is the average  $k$  vector and  $l$  is the sample length,  $\varphi$ , which is the twist angle, and birefringence  $\beta = \pi l(n_e - n_o)/\lambda = gl$ , where  $g = \frac{1}{2}(k^e - k^o)$ . Additional parameter  $X$  is defined as  $X = \sqrt{\varphi^2 + \beta^2}$ .

Therefore, the pump polarization at a position  $z$  in the sample (it travels from  $-L$  to  $z$  so effective length is  $z + L$ ) is transformed according to

$$\begin{pmatrix} e_p^e(z) \\ e_p^o(z) \end{pmatrix} = e^{i\tilde{k}_p(z+L)} M\left(\frac{z+L}{L}\varphi, (z+L)g_p\right) R(\varphi_0) \begin{pmatrix} e_p^H \\ e_p^V \end{pmatrix} \quad (19)$$

where the assumption that the molecules are twisting with a linear gradient is made and  $\varphi$  now denotes

the full twist of the sample. In this case, there is no need for rotation matrix  $R$  from eq. (18) as the state is left in the local coordinate system.

By performing this calculation the following result follows

$$\begin{aligned} e_p^e(z) &= [t_p e_p^H + r_p e_p^V] e^{i\tilde{k}_p(z+L)} \\ e_p^o(z) &= [t_p^* e_p^V - r_p^* e_p^H] e^{i\tilde{k}_p(z+L)}. \end{aligned} \quad (20)$$

Where, in order to shorten the expressions, the following notation is introduced:

$$\begin{aligned} t_p &= \xi_p \cos \varphi_0 - \mu_p \sin \varphi_0 \\ r_p &= \xi_p \sin \varphi_0 + \mu_p \cos \varphi_0 \\ \xi_p &= \cos\left(\frac{z+L}{L} X_p\right) + i \frac{g_p L}{X_p} \sin\left(\frac{z+L}{L} X_p\right) \\ \mu_p &= \frac{\varphi}{X_p} \sin\left(\frac{z+L}{L} X_p\right) \\ X_p &= \sqrt{\varphi^2 + (g_p L)^2} \end{aligned} \quad (21)$$

The logic behind the propagation of signal and idler photons is similar. The only difference is that initially their polarizations are written in the local coordinate system and need to be transformed back into the global system once they exit the sample. This transformation can be written as

$$\begin{pmatrix} e_{s,i}^H \\ e_{s,i}^V \end{pmatrix} = R(-\varphi_0 - \varphi) e^{i\tilde{k}_{s,i}(-z)} M\left(\frac{-z}{L}\varphi, -zg_{s,i}\right) \begin{pmatrix} e_{s,i}^e(z) \\ e_{s,i}^o(z) \end{pmatrix} \quad (22)$$

where the photons are propagating from  $z$  to 0, thus the propagation length is  $-z$  (which is positive due to  $z$  being defined from  $-L$  to 0). The end result can be obtained through the same procedure and yields the following:

$$\begin{aligned} e_{s,i}^H &= [t_{s,i} e_{s,i}^e(z) + r_{s,i} e_{s,i}^o(z)] e^{-i\tilde{k}_{s,i}z} \\ e_{s,i}^V &= [t_{s,i}^* e_{s,i}^o(z) - r_{s,i}^* e_{s,i}^e(z)] e^{-i\tilde{k}_{s,i}z}, \end{aligned} \quad (23)$$

with similar notation as before

$$\begin{aligned}
t_{s,i} &= \xi_{s,i} \cos(\varphi_0 + \varphi) + \mu_{s,i}^* \sin(\varphi_0 + \varphi) \\
r_{s,i} &= -\xi_{s,i}^* \sin(\varphi_0 + \varphi) + \mu_{s,i} \cos(\varphi_0 + \varphi) \\
\xi_{s,i} &= \cos\left(\frac{-z}{L} X_{s,i}\right) + i \frac{g_{s,i} L}{X_{s,i}} \sin\left(\frac{-z}{L} X_{s,i}\right) \\
\mu_p &= \frac{\varphi}{X_{s,i}} \sin\left(\frac{-z}{L} X_{s,i}\right) \\
X_{s,i} &= \sqrt{\varphi^2 + (g_{s,i} L)^2}.
\end{aligned} \tag{24}$$

With these transformations everything is ready for performing the convolution with the nonlinear tensor (eq. 16) that yields the coefficients in the polarization state wavefunction (eq. 15). The only thing left is to conjugate and modify equation (23), to express  $e_{s,i}^{e,o}(z)$  as functions of the outcome polarizations  $e_{s,i}^{H,V}$ :

$$\begin{aligned}
e_{s,i}^e(z) &= [t_{s,i} e_{s,i}^{H*} - r_{s,i}^* e_{s,i}^{V*}] e^{-i\tilde{k}_{s,i} z} \\
e_{s,i}^o(z) &= [r_{s,i} e_{s,i}^{H*} + t_{s,i}^* e_{s,i}^{V*}] e^{-i\tilde{k}_{s,i} z}.
\end{aligned} \tag{25}$$

With equations (16), (20) and (25) the convolution is written as

$$\begin{aligned}
\chi^{(2)} \vec{e}_s^* \vec{e}_i^* \vec{e}_p &= \left[ (r_s e_s^{H*} + t_s^* e_s^{V*}) (r_i e_i^{H*} + t_i^* e_i^{V*}) P_1 + (t_s e_s^{H*} - r_s^* e_s^{V*}) (t_i e_i^{H*} - r_i^* e_i^{V*}) P_2 \right. \\
&\quad \left. + (t_s e_s^{H*} - r_s^* e_s^{V*}) (r_i e_i^{H*} + t_i^* e_i^{V*}) P_3 + (r_s e_s^{H*} + t_s^* e_s^{V*}) (t_i e_i^{H*} - r_i^* e_i^{V*}) P_3 \right] \\
&\quad e^{i\tilde{k}_p L} e^{i[\tilde{k}_p - (\tilde{k}_s + \tilde{k}_i)]z}
\end{aligned} \tag{26}$$

where further notation shortening was introduced via

$$\begin{aligned}
P_1 &= d_{22} (t_p^* e_p^V - r_p^* e_p^H) + d_{32} (t_p e_p^H + r_p e_p^V) \\
P_2 &= d_{23} (t_p^* e_p^V - r_p^* e_p^H) + d_{33} (t_p e_p^H + r_p e_p^V) \\
P_3 &= d_{24} (t_p^* e_p^V - r_p^* e_p^H) + d_{34} (t_p e_p^H + r_p e_p^V).
\end{aligned} \tag{27}$$

This is now the final calculation. The only thing which is left is to integrate this expression over the entire sample (eq. 15) (i.e. take into account contributions from all the slices) and group together the terms which contain the same polarization state of the photon pairs, which yields the corresponding coefficients in the polarization wavefunction (equation 14). For instance, all the terms with  $e_s^{H*} e_i^{H*}$  contribute to the coefficient  $c_1$ . The final result can therefore be written as

$$\begin{aligned}
c_1 &= \int_{-L}^0 dz \left[ r_s r_i P_1 + t_s t_i P_2 + (t_s r_i + r_s t_i) P_3 \right] e^{i[\tilde{k}_p - (\tilde{k}_s + \tilde{k}_i)]z} \\
c_2 &= \int_{-L}^0 dz \left[ (r_s t_i^* + t_s^* r_i) P_1 - (t_s r_i^* + r_s^* t_i) P_2 + (t_s t_i^* - r_s r_i^* + t_s^* t_i - r_s^* r_i) P_3 \right] e^{i[\tilde{k}_p - (\tilde{k}_s + \tilde{k}_i)]z} \\
c_3 &= \int_{-L}^0 dz \left[ t_s^* t_i^* P_1 + r_s^* r_i^* P_2 - (t_s^* r_i^* + r_s^* t_i^*) P_3 \right] e^{i[\tilde{k}_p - (\tilde{k}_s + \tilde{k}_i)]z}
\end{aligned} \tag{28}$$

In order to really obtain the state, the wavefunction has to be normalized. However, when the generation efficiency between different configurations needs to be compared, the norm itself is the parameter by which this can be quantified (in relative terms of course). It has to be noted that the model is much simplified and that many assumptions are made. Still, the model proved to be reliable and provides a great insight into the physics of these kind of materials.

## MISSING SECTIONS

- Experimental setup and SPDC measurements
- Protocol for transforming tomography data into density matrix
- maxLi method
- Measurement of spectrum
- ...

## SUPPLEMENTARY FIGURES

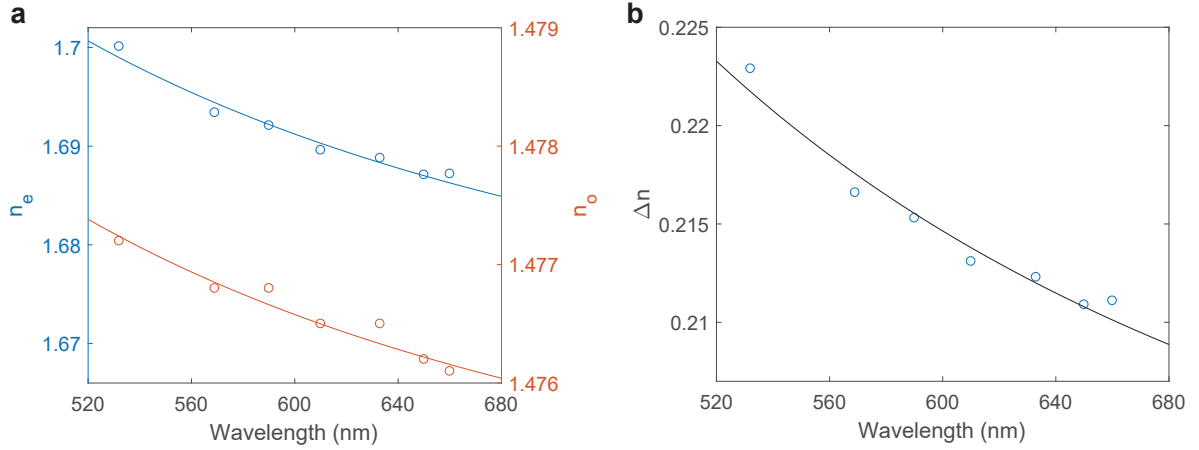

**Figure 2:** Measured values of refractive index, birefringence and wavelength dispersion of the ferroelectric liquid crystal material. **a)** Values and fitted function for both ordinary (right axis) and extraordinary (left axis) refractive index at different wavelengths. **b)** From data in **a**, the values of birefringence can also be extracted. In all cases the fitted functions for dispersion are two-term Cauchy models.

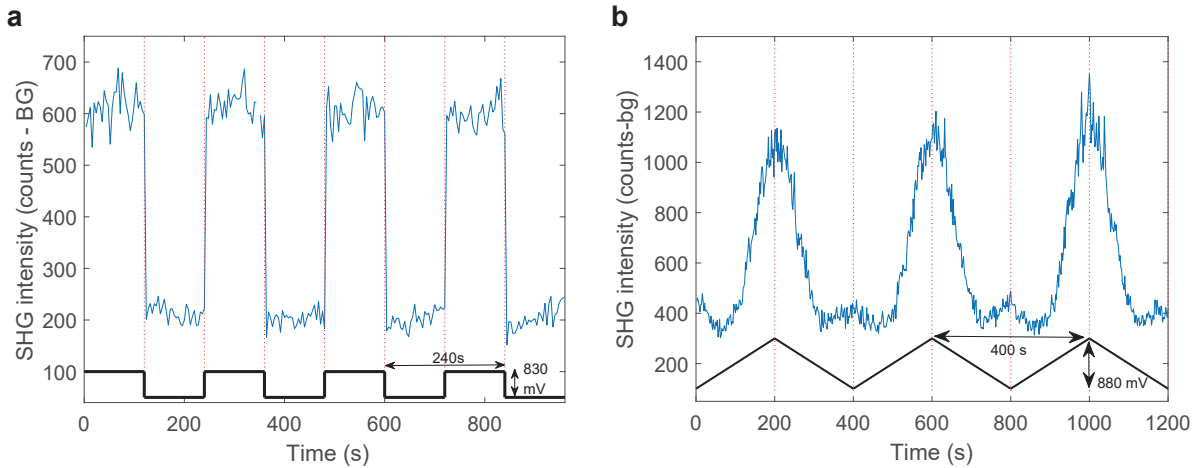

**Figure 3:** Measuring SHG intensity from ferroelectric liquid crystal samples with twist structure for different applied electric fields. **a)** Background subtracted SHG intensity over time while applying square 830mV voltage pulses. We can see discrete transitions when the field is either applied or turned off and stable behavior once the field remains fixed. The contrast between the on and off state of the field is quite large as we see a threefold increase in intensity. **b)** Background subtracted SHG intensity over time while applying linearly increasing/decreasing 880mV voltage pulses. We can see that SHG intensity nicely follows the voltage profile with the only exception being the regions with low voltages where the intensity is not really changing within the measurement error. We can attribute this to the fact that electric field is not sufficient to reorient the molecules and change the sample structure. The contrast between the on and off state of the field is again of the order of three.

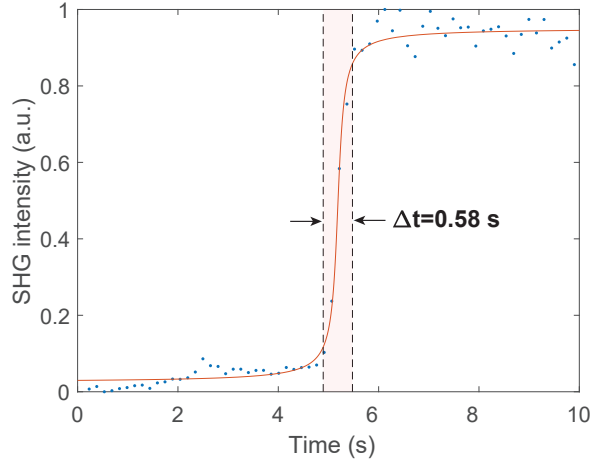

**Figure 4:** Characteristic profile of SHG intensity for a sudden rise in voltage. The transition time in which the molecules reorient and relax into the new configuration driven by the applied field is around half a second. In the presented case, 1 V was applied on the sample without the twist. No significant difference was observed for different field strengths or sample configurations (twist). The same behavior occurs also for SPDC.

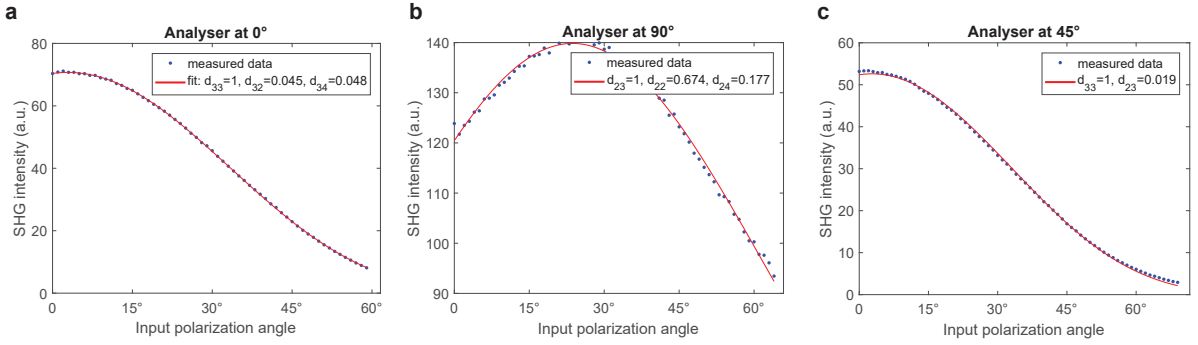

**Figure 5:** Measurements of second order nonlinear tensor resulting in determination of the relative intensities for 6 different components of the effective  $d$  tensor. The reconstructed components are the ones relevant in this work. Due to uniaxial nature of the molecules, the nonlinear tensor should not depend on the rotations around the long molecule axis, which means another set of 6 components will be the same as the measured ones due to sample symmetry. The results are obtained from fitting the SHG intensity at different input polarization angles with respect to the direction of the molecule axis and three different orientations of the analyzer, namely  $0$  ( **a** ),  $\pi/2$  ( **b** ) and  $\pi/4$  ( **c** ). The measurement were performed on several positions across the sample, resulting in the following values for the components (normalized to  $d_{33}$ ) :  $d_{33} = 1$ ,  $d_{32} = 0.070 \pm 0.024$ ,  $d_{34} = 0.029 \pm 0.010$ ,  $d_{23} = 0.052 \pm 0.040$ ,  $d_{22} = 0.047 \pm 0.040$ ,  $d_{24} = 0.007 \pm 0.005$ .

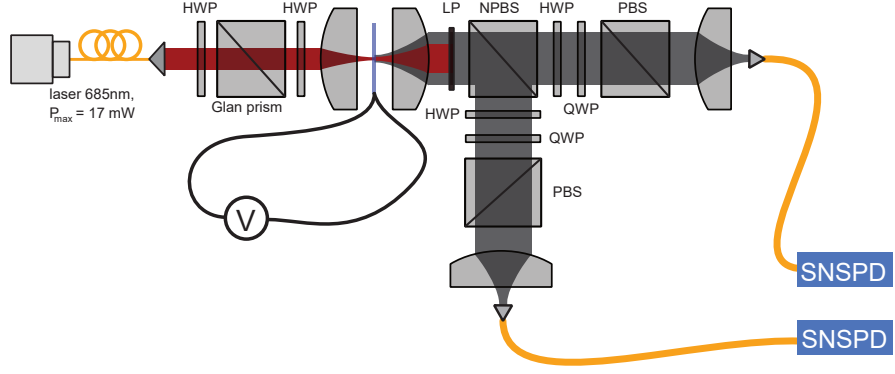

**Figure 6:** Scheme of the measurement setup. A couple of superconducting nanowire single-photon detectors are used in a Hanbury-Brown – Twiss configuration to measure the temporal statistics of arriving photons. Additional optical elements are used to perform polarization tomography and reconstruction of the state.

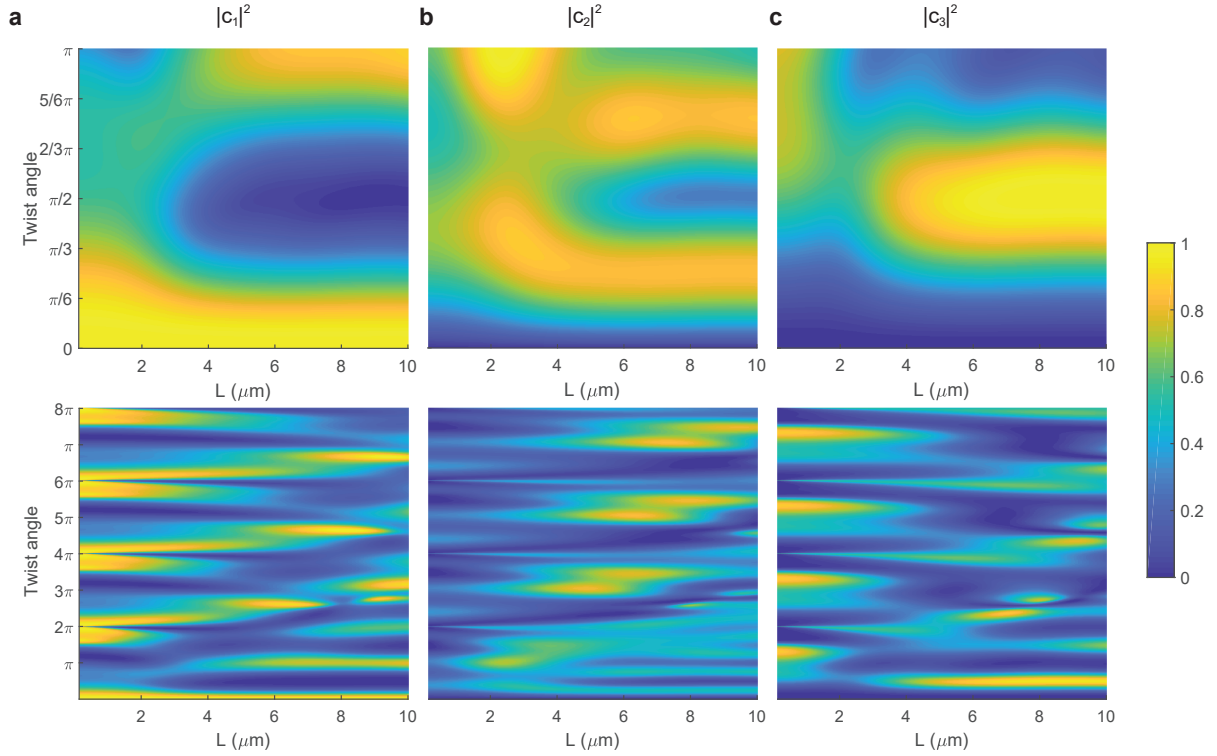

**Figure 7:** Theoretical calculations regarding the polarization state of photon pairs. The squared amplitudes represent the probability for each of the basis states. **a)** Values of  $|c_1|^2$  component over the phase space of sample thickness and twist angle is presented. The same is presented for  $|c_2|^2$  (**b**) and  $|c_3|^2$  component (**c**). In the top panels, the region related to the current experiment is presented, while the bottom panels are plotted for larger twist angles, namely rotations up to 4 full twist, which paves the way for future applications of exploiting these sources for generating arbitrary and highly efficient states.  $D$  pump polarization was used in the calculations.

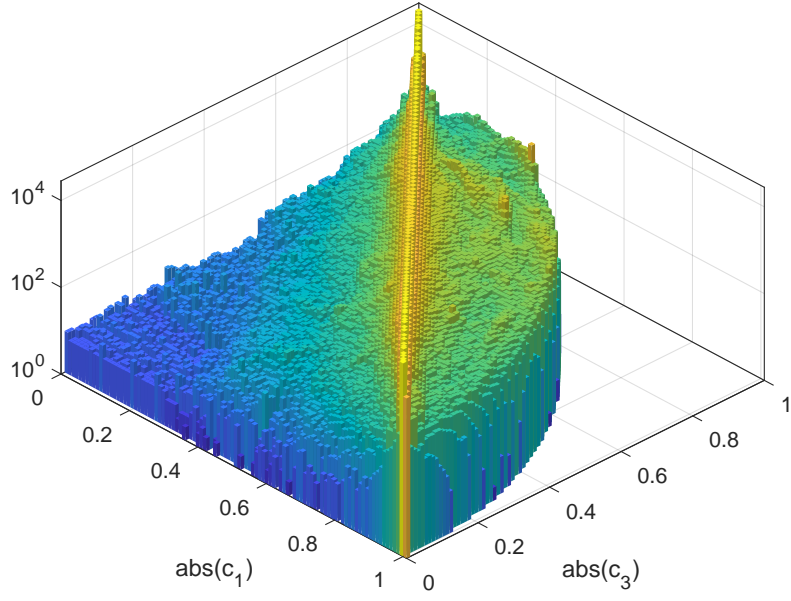

**Figure 8:** Density of the generated states presented in terms of the absolute values of  $c_1$  and  $c_3$  component ( $c_2$  is then defined from normalization condition). It can be seen, that virtually any state can be generated. Sample length up to  $40\text{ }\mu\text{m}$  and twist angle up to  $8\pi$  is used in the simulation as well as 6 different pump polarizations, namely  $H, V, A, D, R$  and  $L$ .

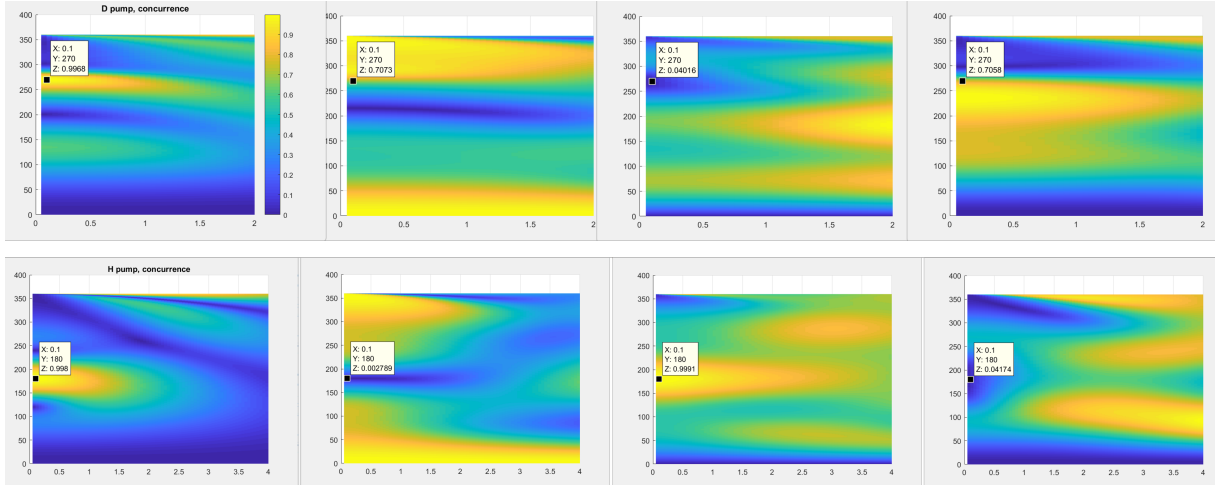

H pump – HV state

| Thickness         | Twist angle | Concurrence | $\text{abs}(c_1)$ | $\text{abs}(c_2)$ | $\text{abs}(c_3)$ |
|-------------------|-------------|-------------|-------------------|-------------------|-------------------|
| 0.2 $\mu\text{m}$ | 180°        | 0.998       | 0.0028            | 0.9991            | 0.0417            |
| 0.5 $\mu\text{m}$ | 179°        | 0.970       | 0.0189            | 0.9865            | 0.1625            |
| 1.0 $\mu\text{m}$ | 175°        | 0.868       | 0.0806            | 0.9494            | 0.3303            |

D pump – HH+VV state

| Thickness         | Twist angle | Concurrence | $\text{abs}(c_1)$ | $\text{abs}(c_2)$ | $\text{abs}(c_3)$ |
|-------------------|-------------|-------------|-------------------|-------------------|-------------------|
| 0.2 $\mu\text{m}$ | 270°        | 0.997       | 0.7073            | 0.0402            | 0.7058            |
| 0.5 $\mu\text{m}$ | 268.5°      | 0.952       | 0.6837            | 0.1541            | 0.7133            |
| 1.0 $\mu\text{m}$ | 262.5°      | 0.815       | 0.6101            | 0.3046            | 0.7314            |

**Figure 9:** HH+VV state and HV state (maximally entangled states) can be almost perfectly realized with given sample configuration. These states can then easily be transformed into standard HH or VV state by applying electric field in a given direction. (NOT FINISHED)

## 1 References

- [1] Hiroya Nishikawa, Kazuya Shiroshita, Hiroki Higuchi, Yasushi Okumura, Yasuhiro Haseba, Shin-ichi Yamamoto, Koki Sago, and Hirotugu Kikuchi. A fluid liquid-crystal material with highly polar order. *Advanced materials*, 29(43):1702354, 2017.
- [2] Nerea Sebastián, Martin Čopič, and Alenka Mertelj. Ferroelectric nematic liquid-crystalline phases. *Physical Review E*, 106(2):021001, 2022.
- [3] Xi Chen, Vikina Martinez, Eva Korblova, Guillaume Freychet, Mikhail Zhernenkov, Matthew A Glaser, Cheng Wang, Chenhui Zhu, Leo Radzihovsky, Joseph E MacLennan, et al. The smectic za phase: Antiferroelectric smectic order as a prelude to the ferroelectric nematic. *Proceedings of the National Academy of Sciences*, 120(8):e2217150120, 2023.

- [4] Xi Chen, Eva Korblova, Dengpan Dong, Xiaoyu Wei, Renfan Shao, Leo Radzihovsky, Matthew A Glaser, Joseph E MacLennan, Dmitry Bedrov, David M Walba, et al. First-principles experimental demonstration of ferroelectricity in a thermotropic nematic liquid crystal: Polar domains and striking electro-optics. *Proceedings of the National Academy of Sciences*, 117(25):14021–14031, 2020.
- [5] Nerea Sebastián, Richard J Mandle, Andrej Petelin, Alexey Eremin, and Alenka Mertelj. Electrooptics of mm-scale polar domains in the ferroelectric nematic phase. *Liquid Crystals*, 48(14):2055–2071, 2021.
- [6] Jeong-Seon Yu, Jae Hoon Lee, Jun-Yong Lee, and Jong-Hyun Kim. Alignment properties of a ferroelectric nematic liquid crystal on the rubbed substrates. *Soft Matter*, 19(13):2446–2453, 2023.
- [7] Amnon Yariv and Pochi Yeh. Optical waves in crystal propagation and control of laser radiation. 1983.
- [8] Ignacio Moreno, Nouredine Bennis, Jeffrey A Davis, and Carlos Ferreira. Twist angle determination in liquid crystal displays by location of local adiabatic points. *Optics communications*, 158(1-6):231–238, 1998.
- [9] Kanghua Lu and Bahaa EA Saleh. Theory and design of the liquid crystal tv as an optical spatial phase modulator. *Optical Engineering*, 29(3):240–246, 1990.
